# Supplementary material for: Validation of the GreenX library time-frequency component for efficient GW and RPA calculations
Source: arXiv:2403.06709 ancillary file (2024-03-12)
Supplement: Supplementary file 1 [file Supplemental_Material.pdf]

# Supplemental Material for "Validation of the GreenX library time-frequency component for efficient $GW$ and RPA calculations"

Maryam Azizi,[1] Jan Wilhelm,[2] Dorothea Golze,[3] Francisco A. Delesma,[3,4] Ramón L. Panadés-Barrueta,[3] Patrick Rinke,[4] Matteo Giantomassi,[1] and Xavier Gonze[1]

[1] *Université Catholique de Louvain, Louvain-la-Neuve, Belgium*

[2] *Institute of Theoretical Physics and Regensburg Center for Ultrafast Nanoscopy (RUN), University of Regensburg, Regensburg, Germany*

[3] *Faculty for Chemistry and Food Chemistry, Technische Universität Dresden, 01062 Dresden, Germany*

[4] *Department of Applied Physics, Aalto University, FI-02150 Espoo, Finland*

(Dated: March 11, 2024)

## I. CONVENTIONAL RPA ENERGIES

TABLE S1. RPA total energy [eV] of the $H_2O$ molecule calculated using the Gauss-Legendre, modified Gauss-Legendre and minimax imaginary frequency points

| n | Gauss-Legendre | modified Gauss-Legendre | minimax |
|---|---|---|---|
| 06 | -2077.993515947127434629 | -2079.618349892663445644 | -2079.573216833881815546 |
| 08 | -2079.470897121835150756 | -2079.651398894266094430 | -2079.569968952466751944 |
| 10 | -2079.793015335706058977 | -2079.588204814459913905 | -2079.569988196195481578 |
| 12 | -2079.726706347793879104 | -2079.552815249955074250 | -2079.569984253739676205 |
| 14 | -2079.624885226010064798 | -2079.552679979373351671 | -2079.569984899238988874 |
| 16 | -2079.569593949986028747 | -2079.562052879844031850 | -2079.569984883855795488 |
| 18 | -2079.551407504082362721 | -2079.568647285111637757 | -2079.569984886807560542 |
| 20 | -2079.549571590699542867 | -2079.571074691903049825 | -2079.569984886582460604 |
| 22 | -2079.552252733752993663 | -2079.571184255757543724 | -2079.569984886643851496 |
| 24 | -2079.555266937161832175 | -2079.570628251328798797 | -2079.569984886622478371 |
| 26 | -2079.557735171345484559 | -2079.570169948059628950 | -2079.569984886596557772 |
| 28 | -2079.559662190994004050 | -2079.569960252885266527 | -2079.569984886596557772 |
| 30 | -2079.561162685470208089 | -2079.569916817083594651 | -2079.569984886595193530 |
| 32 | -2079.562333148364359658 | -2079.569937758221385593 | -2079.569984886599741003 |
| 34 | -2079.563255232028495811 | -2079.569965656914064311 | -2079.569984886598376761 |
| 36 | -2079.563997345932421013 | -2079.569982162646738288 | |
| 38 | -2079.564610708895997959 | -2079.569987837977805611 | |
| 40 | -2079.565129407349104440 | -2079.569987949323603971 | |
| 42 | -2079.565574818307595706 | -2079.569986525245440134 | |
| 44 | -2079.565960826011178142 | -2079.569985366581477138 | |
| 46 | -2079.566297487130668742 | -2079.569984829363875178 | |
| 48 | -2079.566592846224921232 | -2079.569984713838493917 | |
| 50 | -2079.566853574822289374 | -2079.569984765912977309 | |

TABLE S2. RPA total energy [eV] of the MgO bulk system calculated using the Gauss-Legendre, modified Gauss-Legendre and minimax imaginary frequency points

| n | Gauss-Legendre | modified Gauss-Legendre | minimax |
|---|---|---|---|
| 06 | -7505.960780090952539467 | -7508.914243757246367749 | -7509.026794604134011024 |
| 08 | -7508.021027612132456852 | -7509.266485370255395537 | -7508.985063619610627938 |
| 10 | -7508.944250255097358603 | -7509.216039447337607271 | -7508.987416438678337726 |
| 12 | -7509.189252190359184169 | -7509.074424665955120872 | -7508.987611024338548304 |
| 14 | -7509.153441584454412804 | -7508.982064574450305372 | -7508.987566337910720903 |
| 16 | -7509.060388210873497882 | -7508.949089252736484922 | -7508.987569136581441853 |
| 18 | -7508.991062242549560323 | -7508.950534801747380697 | -7508.987569321961927926 |
| 20 | -7508.956931049589911708 | -7508.963892869467599666 | -7508.987569330574842751 |
| 22 | -7508.947313052360186702 | -7508.976949045193578058 | -7508.987569328913195931 |
| 24 | -7508.949777328392883646 | -7508.985454501069398247 | -7508.987569328937752288 |
| 26 | -7508.956079853030132653 | -7508.989387419885133567 | -7508.987569328853169281 |
| 28 | -7508.962236569136621255 | -7508.990268664624636585 | -7508.987569328848621807 |
| 30 | -7508.966978844782715896 | -7508.989697221149071992 | -7508.987569328840436355 |
| 32 | -7508.970312182223096897 | -7508.988769755694193008 | -7508.987569328846802818 |
| 34 | -7508.972631699967678287 | -7508.988021775416200398 | -7508.987569328837707871 |
| 36 | -7508.974322524857598182 | -7508.987593718235075357 | |
| 38 | -7508.975645795841955987 | -7508.987429109750337374 | |
| 40 | -7508.976747885781151126 | -7508.987417121696125832 | |
| 42 | -7508.977701474003879411 | -7508.987464767180426861 | |
| 44 | -7508.978541130111807433 | -7508.987517628451314521 | |
| 46 | -7508.979284996443311683 | -7508.987554183696374821 | |
| 48 | -7508.979945251719072985 | -7508.987572317966623813 | |
| 50 | -7508.980532086746279674 | -7508.987577655976565438 | |

TABLE S3. RPA total energy [eV] of the Thiel set of small organic molecules calculated using the modified Gauss-Legendre grid ($\omega = 200$) and minimax grids ($\omega = 10, 20, 30$)

| n | System | minimax $\omega = 10$ | minimax $\omega = 20$ | minimax $\omega = 30$ | mod-GL $\omega = 200$ |
|---|---|---|---|---|---|
| 1 | Ethene | -2140.914727913780 | -2140.914716357730 | -2140.914716357710 | -2140.914716357120 |
| 2 | Butadiene | -4248.726296682890 | -4248.726294548760 | -4248.726294548770 | -4248.726294545620 |
| 3 | Hexatriene | -6356.570202258350 | -6356.570433819740 | -6356.570433819120 | -6356.570433813510 |
| 4 | Octatetraene | -8464.425743549560 | -8464.426268958450 | -8464.426268957370 | -8464.426268950370 |
| 5 | Cyclopropene | -3176.163767789950 | -3176.163800684260 | -3176.163800684310 | -3176.163800682650 |
| 6 | Cyclopentadiene | -5286.106967500870 | -5286.106993986120 | -5286.106993986100 | -5286.106993981840 |
| 7 | Norbornadiene | -7393.617978015450 | -7393.617918584810 | -7393.617918584830 | -7393.617918574850 |
| 8 | Benzene | -6324.317297662750 | -6324.317362654430 | -6324.317362654450 | -6324.317362648620 |
| 9 | Naphthalene | -10507.478422201300 | -10507.478833826200 | -10507.478833824900 | -10507.478833816200 |
| 10 | Furan | -6262.715720268450 | -6262.715625320050 | -6262.715625320020 | -6262.715625315860 |
| 11 | Pyrrole | -5722.923630015730 | -5722.923673688940 | -5722.923673688950 | -5722.923673684650 |
| 12 | Imidazole | -6159.257770027380 | -6159.257800446020 | -6159.257800446020 | -6159.257800440970 |
| 13 | Pyridine | -6760.346069270210 | -6760.346027043490 | -6760.346027043560 | -6760.346027038540 |
| 14 | Pyrazine | -7196.233928499770 | -7196.234092691490 | -7196.234092691120 | -7196.234092686550 |
| 15 | Pyrimidine | -7196.432826875760 | -7196.432953603950 | -7196.432953603340 | -7196.432953598230 |
| 16 | Pyridazine | -7195.460835602170 | -7195.461084549230 | -7195.461084548880 | -7195.461084542900 |
| 17 | Triazine | -7632.592140304250 | -7632.592186874540 | -7632.592186874460 | -7632.592186869480 |
| 18 | Tetrazine | -8066.538170070050 | -8066.538610722330 | -8066.538610720680 | -8066.538610714780 |
| 19 | Formaldehyde | -3117.447970402200 | -3117.448004522970 | -3117.448004522860 | -3117.448004522360 |
| 20 | Acetone | -5260.022923409990 | -5260.022983837730 | -5260.022983837570 | -5260.022983835240 |
| 21 | Benzoquinone | -10384.498468349900 | -10384.498731071900 | -10384.498731068000 | -10384.498731061500 |
| 22 | Formamide | -4625.482833177200 | -4625.482790691840 | -4625.482790691890 | -4625.482790689750 |
| 23 | Acetamide | -5696.702018177720 | -5696.701954184210 | -5696.701954184120 | -5696.701954181690 |
| 24 | Propanamide | -6767.757593888080 | -6767.757506082310 | -6767.757506082410 | -6767.757506076430 |
| 25 | Cytosine | -10751.835096198500 | -10751.835227359300 | -10751.835227358400 | -10751.835227350400 |
| 26 | Thymine | -12363.716621210000 | -12363.716772287300 | -12363.716772286600 | -12363.716772277700 |
| 27 | Uracil | -11292.522255841900 | -11292.522370221600 | -11292.522370221100 | -11292.522370213700 |
| 28 | Adenine | -12722.451675503900 | -12722.451784160500 | -12722.451784160500 | -12722.451784152600 |

TABLE S4. RPA total energy [eV] of crystalline systems calculated using the modified Gauss-Legendre grid ($\omega$ = 200) and minimax grids ($\omega = 10, 20, 30$)

| n | System | minimax $\omega = 10$ | minimax $\omega = 20$ | minimax $\omega = 30$ | mod-GL $\omega = 200$ |
|---|---|---|---|---|---|
| 1 | Si | -15798.1027218825 | -15798.1132251371 | -15798.1132251704 | -15798.1132251806 |
| 2 | LiF | -2931.6325963727 | -2931.6327180603 | -2931.6327180603 | -2931.6327180749 |
| 3 | SiC | -8939.3312244539 | -8939.3295690583 | -8939.3295690801 | -8939.3295690991 |
| 4 | C | -2078.0871660422 | -2078.0872330553 | -2078.0872330552 | -2078.0872330776 |
| 5 | BN | -2174.3380977894 | -2174.3380420364 | -2174.3380420361 | -2174.3380420509 |
| 6 | MgO | -7508.9874157272 | -7508.9875693305 | -7508.9875693288 | -7508.9875693450 |
| 7 | GaAs | -115038.7600053269 | -115038.7756207713 | -115038.7756193425 | -115038.7756193615 |

## II. LOW-SCALING GW FOR MOLECULES AND SOLIDS

TABLE S5. Convergence of HOMO and LUMO energies of the GW100 benchmark set computed with the low-scaling algorithm at the $G_0W_0$@PBE level as a function of the number of minimax points N.

| | MAD (eV) | | AD $\leq$ 0.01 eV | | AD $\leq$ 0.02 eV | |
|---|---|---|---|---|---|---|
| N | HOMOs | LUMOs | HOMOs | LUMOs | HOMOs | LUMOs |
| 10 | 0.11 | 0.091 | 15 | 18 | 30 | 34 |
| 12 | 0.087 | 0.010 | 30 | 41 | 48 | 79 |
| 14 | 0.065 | 0.017 | 27 | 60 | 40 | 84 |
| 16 | 0.038 | 0.019 | 29 | 53 | 41 | 73 |
| 18 | 0.032 | 0.008 | 28 | 62 | 49 | 91 |
| 20 | 0.025 | 0.011 | 28 | 66 | 60 | 94 |
| 22 | 0.020 | 0.011 | 47 | 79 | 75 | 92 |
| 24 | 0.013 | 0.008 | 70 | 87 | 86 | 94 |
| 26 | 0.016 | 0.008 | 70 | 90 | 83 | 95 |
| 28 | 0.006 | 0.006 | 84 | 93 | 90 | 96 |
| 30 | 0.008 | 0.004 | 87 | 97 | 92 | 100 |
| 32 | 0.008 | 0.008 | 85 | 96 | 92 | 98 |

TABLE S6. $G_0W_0$@LDA band gap [eV] of 2D materials using 10, 20 and 30 minimax points ($N$)

| $N$ | $MoS_2$ | $MoSe_2$ | $WS_2$ | $WSe_2$ |
|---|---|---|---|---|
| 10 | 2.455 | 2.053 | 2.793 | 2.347 |
| 20 | 2.476 | 2.074 | 2.814 | 2.362 |
| 30 | 2.471 | 2.071 | 2.812 | 2.367 |

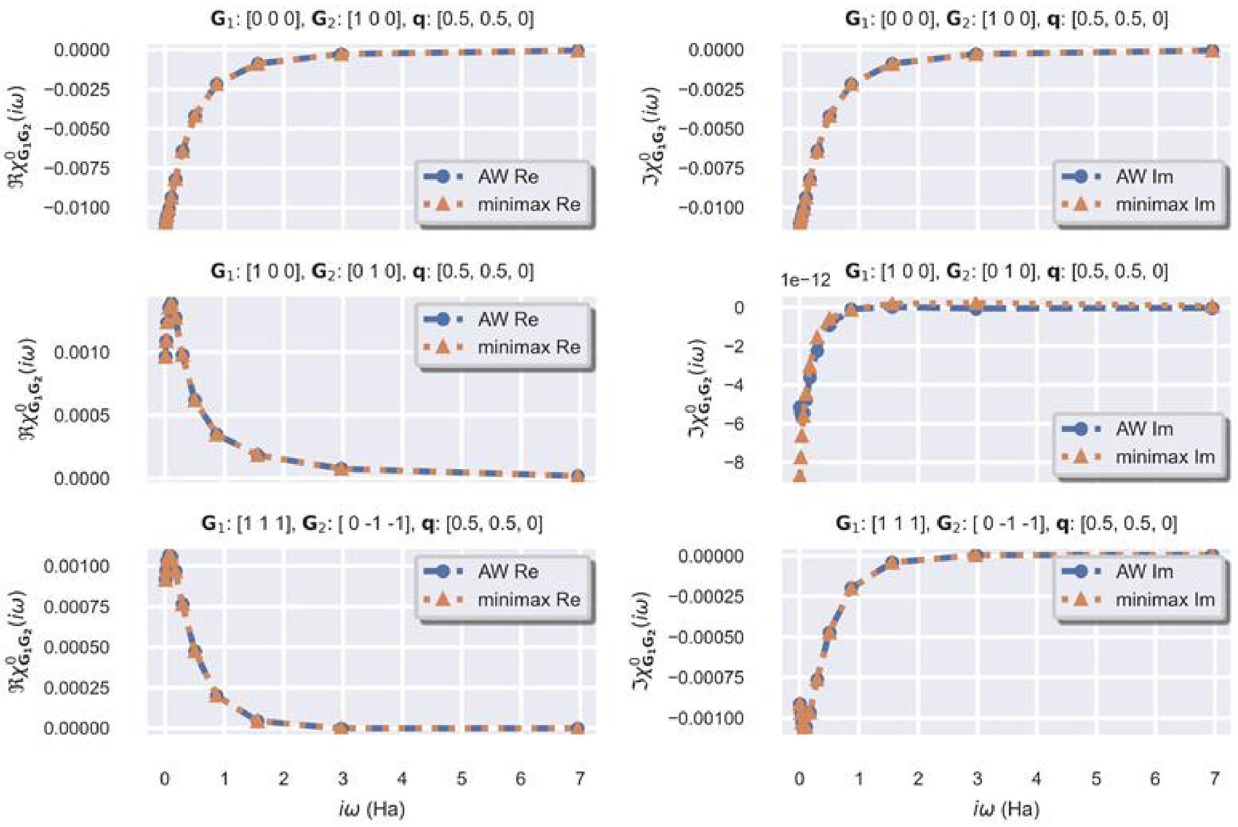


FIG. S1. Selected matrix elements of the susceptibility of silicon, as a function of the frequency on the imaginary axis. They are calculated using Adler-Wiser formula Eq.(4) (blue) and the real space imaginary-time minimax method (orange), with excellent agreement. The left column shows the real part of the susceptibility, and the right column shows the imaginary part of the susceptibility. Note the vertical scale of the middle right figure, that is to be multiplied by the indicated $10^{-12}$ factor.

TABLE S7. Conventional and Low-scaling GW results for the selected benchmark system using ABINIT. For the low-scaling calculations the results have been reported for 10, 20 and 30 grid points.

| | | Conventional GW (eV) | Low-scaling GW (eV) | | |
|---|---|---|---|---|---|
| | | | 10 | 20 | 30 |
| 1 | Si | 3.238 | 3.267 | 3.248 | 3.248 |
| 2 | LiF | 13.836 | 14.013 | 13.84 | 13.842 |
| 3 | SiC | 7.323 | 7.399 | 7.325 | 7.325 |
| 4 | C | 7.371 | 7.391 | 7.371 | 7.372 |
| 5 | BN | 11.153 | 11.295 | 11.153 | 11.158 |
| 6 | MgO | 7.216 | 7.235 | 7.219 | 7.221 |
| 7 | GaAs | 0.748 | 0.762 | 0.758 | 0.758 |
